# Supplementary material for: Solving Infinite-State Games via Acceleration (Full Version)
Source: arXiv:2305.16118 source file (2023-11-07)
Supplement: Supplementary file 1 [file appendix-parity.tex]

For a reactive program game structure $\mathcal G = (T,\inputs, \cells, L, \Inv, \delta)$ and location invariant $\Inv': L \to \FOL{V}$ we define $\mathcal G[\Inv']:=(T,\inputs, \cells, L, \Inv', \delta)$ to be the reactive program game structure obtained by replacing $\Inv$ by $\Inv'$, under the assumption that $\Inv'$ induces a well-defined game structure.

\begin{figure}[h!]
\begin{algorithm}[H]
    \SetKwProg{Fn}{function}{}{}
    \DontPrintSemicolon
    \Fn{\textsc{SolveParityGame}($\mathcal G = (T,\inputs, \cells, L, \Inv, \delta)$,  $\mathit{col} : L \to \{0, 1, \dots k\}$)}{          
       \nl \lIf{$\mathit{Inv} \equiv_{T} \lambda l.~\bot$}
                 {\Return $(\lambda l.~\bot,\lambda l.~\bot)$}
	   \nl $m$ := $\max \{c \in  \{0, 1, \dots k \} \mid \exists l \in L.~\mathit{col}(l) = c \text{ and } \sat{\mathit{Inv}(l)}\}$\;
	  \tcc{If the maximum color is $0$,  Player \sys\ trivially wins.}
	  \nl  \lIf{$m=0$}{\Return $(\mathit{Inv},\lambda l.~\bot)$}     
	  \nl \lIf{$m \mod 2 = 0$}{$p$ := $\sys$ \textbf{ else }$p$ := $\env$} 
      \tcc{$L_m$ is the set of locations with color $m$.}
	  \nl $L_m$ := $\{l \in L \mid \mathit{col}(l) = m \text{ and } \sat{\mathit{Inv}(l)}\}$\;
      \nl $a$ :=  \textsc{Attractor}($\mathcal G$, $p$,  $\{l \mapsto \Inv (l) \mid l \in L_m\}$)\;
      \nl $(w_{\sys}',w_{\env}')$ := $\textsc{SolveParityGame}(\mathcal G[\mathit{Inv} \wedge \neg a],  \mathit{col})$\; \label{line:rec-1}
      \nl \lIf{$w_{1- p}' \equiv_{T} \lambda l.~\bot$}{
	  	  $\{w_{p}$ := $\mathit{Inv}$;~$w_{1- p}$ := $\mathcal \lambda l.~\bot$;~
		      \Return $(w_{\sys},w_{\env})\}$
      }
      \nl $b$ :=  \textsc{Attractor}($\mathcal G$,  $1- p$,  $w_{1- p}'$)\;                   
      \nl $(w_{\sys}'',w_{\env}'')$ := $\textsc{SolveParityGame}(\mathcal G[\mathit{Inv} \wedge \neg b],  \mathit{col})$\;	   \label{line:rec-2}
   \nl   $w_{p}$ := $w_{p}''$;~
	  $w_{1-p}$ := $w_{1-p}'' \lor b$;~
	  \Return $(w_{\sys},w_{\env})$
    }
\caption{A symbolic semi-algorithm for solving reactive program games with parity objectives.
Given a reactive program game structure  $\mathcal G$ and coloring function $\mathit{col}$, it computes the pair $(w_{\sys},w_{\env}) \in \symstates\times\symstates$ representing the sets of states in $\sema{\mathcal G}$ that are winning for Player \sys\ and Player \env\ respectively in the parity game defined by $\mathcal G$ and $\mathit{col}$.}\label{algo:parity}    
\end{algorithm}
\end{figure}

The procedure \textsc{SolveParityGame} for solving parity games on reactive program game structures is given in Algorithm~\ref*{algo:parity}.  It makes two recursive calls, at lines~\ref*{line:rec-1} and~\ref*{line:rec-2}. 
 
At line~\ref*{line:rec-1} the procedure is called with a game obtained by adding as invariant the negation of the attractor $a$, which, in particular, contains \emph{all the states} with location in $L_m$. Thus, since the number of locations in the game structure is finite, a chain of recursive calls at line~\ref*{line:rec-1} will have finite depth.

The recursive call at line~\ref*{line:rec-2} is with the game structure obtained by adding the invariant $\neg b$, where $b$ consists of states that are winning for Player $1-p$.  

The soundness of Algorithm~\ref*{algo:parity} follows from the correctness of Zielonka's algorithm~\cite{Zielonka98}.
